# Supplementary material for: Gradient-Guided Annealing for Domain Generalization
Source: arXiv:2502.20162 source file (2025-07-21)
Supplement: Supplementary file 2 [file preamble.tex]

%
% --- inline annotations
%
\newcommand{\red}[1]{{\color{red}#1}}
\newcommand{\todo}[1]{{\color{red}#1}}
\newcommand{\TODO}[1]{\textbf{\color{red}[TODO: #1]}}
% --- disable by uncommenting  
% \renewcommand{\TODO}[1]{}
% \renewcommand{\todo}[1]{#1}
